# Supplementary material for: Revisiting DeepFool: generalization and improvement
Source: arXiv:2303.12481 source file (2024-12-08)
Supplement: Supplementary file 1 [file supp.tex]

% \documentclass[10pt,twocolumn,letterpaper]{article}
% \usepackage{iccv}
% \usepackage{times}
% \usepackage{epsfig}
% \usepackage{graphicx}
% \usepackage{amsmath}
% \usepackage{amssymb}
% \usepackage{enumitem}
% \usepackage{subcaption}
% \usepackage{amsthm}
% \usepackage{multirow}
% \usepackage[T1]{fontenc}

% % Recommended, but optional, packages for figures and better typesetting:
% \usepackage{microtype}
% \usepackage{graphicx, xcolor}
% % \usepackage{subfigure}

% \usepackage{booktabs} % for professional tables
% \usepackage{amsmath}
% \usepackage{amssymb}
% \usepackage{mathrsfs}
% \usepackage{subcaption}
% \usepackage{multirow}
% \usepackage{makecell}
% \usepackage{xcolor}
% \usepackage{amssymb}% http://ctan.org/pkg/amssymb
% \usepackage{pifont}% http://ctan.org/pkg/pifont
% \newcommand{\cmark}{\ding{51}}%
% \newcommand{\xmark}{\ding{55}}%
% \newcommand{\theHalgorithm}{\arabic{algorithm}}
% \usepackage{nicematrix}
% \usepackage{xcolor}
% \usepackage{tabularray}
% \usepackage{colortbl}
% \usepackage{mathrsfs}
% \usepackage{color}
% \usepackage{subcaption}
% % \usepackage{footmisc}
% \usepackage[]{algorithm2e}
% \usepackage{makecell}
% \usepackage{multirow}
% \usepackage{fancyhdr}
% \usepackage{appendix}
% \usepackage{textcomp}
% \usepackage{xr}

% \makeatletter
% \newcommand*{\addFileDependency}[1]{% argument=file name and extension
% \typeout{(#1)}% latexmk will find this if $recorder=0
% % however, in that case, it will ignore #1 if it is a .aux or 
% % .pdf file etc and it exists! If it doesn't exist, it will appear 
% % in the list of dependents regardless)
% %
% % Write the following if you want it to appear in \listfiles 
% % --- although not really necessary and latexmk doesn't use this
% %
% \@addtofilelist{#1}
% %
% % latexmk will find this message if #1 doesn't exist (yet)
% \IfFileExists{#1}{}{\typeout{No file #1.}}
% }\makeatother

% \newcommand*{\myexternaldocument}[1]{%
% \externaldocument{#1}%
% \addFileDependency{#1.tex}%
% \addFileDependency{#1.aux}%
% }


% \myexternaldocument{superdeepfool}
% \usepackage[pagebackref=true,breaklinks=true,letterpaper=true,colorlinks,bookmarks=false]{hyperref}

% % \iccvfinalcopy % *** Uncomment this line for the final submission

% \def\iccvPaperID{10790} % *** Enter the ICCV Paper ID here
% \def\httilde{\mbox{\tt\raisebox{-.5ex}{\symbol{126}}}}

% %%%%%%%%%%%%%% Notation %%%%%%
% \def\x{\boldsymbol{x}}
% \def\y{\boldsymbol{y}}
% \def\r{\boldsymbol{r^*}_{adv}(\x)}
% \def\w{\boldsymbol{w}}
% %%%%%%%%%%%%%%%%%%%%%%%%%%%%%%
% \newtheorem{lemma}{Lemma}
% \newtheorem{theorem}{Theorem}
% \newtheorem{proposition}{Proposition}
% % \newtheorem{proof}{Proof}
% %%%%%%%%%%%%%%%%%%%%%%%%%%%%%%%%%%%%%%%%%%%

% \DeclareMathOperator*{\argmin}{arg\,min}
% \DeclareMathOperator*{\argmax}{arg\,max}
% \DeclareMathOperator*{\sign}{sign}
% % \newcolumntype{Y}{>{\centering\arraybackslash}X}
% % \newcolumntype{s}{>{\hsize=.4\hsize}X}
% \newcommand{\olive}[2]{{\color{red}{ #1 }}{\small\color{olive}{ #2 }}}
% \newcommand{\mahed}[2]{{\color{blue}{#1}}{\small\color{blue}{#2}}}

% \newcommand{\cw}{\texttt{C$\&$W}}
% \newcommand{\DF}{\texttt{DF}}
% \newcommand{\DDN}{\texttt{DDN}}
% \newcommand{\project}{\textsf{project}}
% \newcommand{\SDF}{\texttt{SDF}}
% \newcommand{\grad}{\nabla}
% \newcommand{\C}{\mathcal{C}}
% \newcommand{\bbR}{\mathbb{R}}
% \newcommand{\bbN}{\mathbb{N}}
% \newcommand{\E}{\mathbb{E}}
% \newcommand{\std}[1]{\tiny{$\pm$ #1}}



% %%%%%%%%% ICCV %%%%%%%%%%%%%%%
% % Pages are numbered in submission mode, and unnumbered in camera-ready
% \ificcvfinal\pagestyle{empty}\fi

% \begin{document}

% %%%%%%%%% TITLE
% \title{Revisiting DeepFool: generalization and improvement\\Appendix}

% \author{Alireza Abdollahpourrostam\textsuperscript{1}  \hspace{5mm} Mahed Abroshan\textsuperscript{2}  \hspace{5mm} Seyed-Mohsen Moosavi-Dezfooli~\textsuperscript{3}\\
% 	\textsuperscript{1} Tehran Polytechnic, Iran~~\hspace{1mm}
%     \textsuperscript{2} Optum Labs, London, UK~~
% 	\hspace{2mm}\textsuperscript{3} Imperial College London, UK\\
% 	{\tt\small alirezaabdollahpour1380@gmail.com, mahed.abroshan@optum.com,  seyed.moosavi@imperial.ac.uk} \\
% }


% \maketitle
% % Remove page # from the first page of camera-ready.
% \ificcvfinal\thispagestyle{empty}\fi

% \appendix
% \input{appendix}

% \clearpage
% \newpage
% \twocolumn
% {\small
% \bibliographystyle{ieee_fullname}
% \bibliography{egbib}
% }

% \end{document}
